# Supplementary material for: Specification and Implementation of Replicated List: The Jupiter Protocol Revisited
Source: arXiv:1708.04754 source file (2018-11-12)
Supplement: Supplementary file 1 [file statespace2d-edge-version.tex]

% cscw-2d-state-space
\begin{algorithm}
  \caption{2D State Space.}
  \label{cscw-2d-state-space}
  \begin{algorithmic}[1]
    \CLASS{Vertex} 
      \State \VAR{ops} : $2^{\opset} = \emptyset$
      \State \VAR{le} : Edge = \Null{}  \Comment{\todo{remember to update}}
      \State \VAR{ge} : Edge = \Null{}
    \EndClass{Vertex}

    \Statex
    \CLASS{Edge} 
      \State \VAR{u} : Vertex = \Null{}
      \State \VAR{v} : Vertex = \Null{}
      \State \VAR{o}\, : $\opset$ = \Nop{}
      \State \VAR{f} : $\set{l, r}$
    \EndClass{Edge}

    \Statex
    \CLASS{StateSpace2D}
      \State \VAR{init} : Vertex = new Vertex()
      \State \VAR{cur}\ : Vertex = $init$

      \Statex
      \Procedure{LocalProcessing}{$o : \opset$}
	\State Vertex $v \gets$ new Vertex($cur.ops \cup \set{o}$)
	\State Edge $e \gets$ new Edge($cur, v, o, l$)
	\State $cur \gets v$
      \EndProcedure

      \Statex
      \Procedure{RemoteProcessing}{$o : \opset$} : $\opset$
	\State $u \gets$ \Call{Locate}{$o$} \Comment{\todo{no search?}}
	\State Vertex $v \gets$ new Vertex($u.ops \cup \set{o}$)  \Comment{\todo{original op?}}
	\State Edge $e \gets$ new Edge($u, v, o, g$)
	\State $\cdots$ (transform)
	\State $cur \gets \cdots$
      \EndProcedure

      \Statex
      \Procedure{Locate}{$o : \opset$}
      \EndProcedure

      \Statex
      \Procedure{xFormSeq}{$e : $ Edge} : $\opset$  \Comment{\todo{fig!}}
	\State $e.f$  \Comment{\todo{if else?}}
	\While {$(e' \gets e.u.le) \not=$ \Null{}}
	  \State $(\cdots) \gets$ \Call{xForm}{$e.o, e.o'$}
	  \State \textbf{let} $v \gets e.v$
	  \State \textbf{let} $u' \gets e'.v$
	  \State Vertex $v'$ = new Vertex($v.ops \cup \set{e'.o}$)
	  \State Edge $e_{vv'}$ = new Edge($v, v', \cdots, l$)  \Comment{\todo{original?}}
	  \State Edge $e_{u'v'}$ = new Edge($u', v', \cdots, g$)  \Comment{\todo{original?}}
	  \State \textbf{let} $e \gets e_{u'v'}$
	\EndWhile
	\State \Return $e.o$
      \EndProcedure
    \EndClass{StateSpace2D}
  \end{algorithmic}
\end{algorithm}

% \CLASS{Vertex} 
%   \State \VAR{state} : $\set{\text{Op}} = \emptyset$
%   \State \VAR{global} : Vertex = \Null{}%
%   \State \VAR{local}\;\; : Vertex = \Null{}%
%   \State \VAR{global\_op } : Op = \Nop{}%
%   \State \VAR{local\_op}\;\;\; : Op = \Nop{}%
% \EndClass{Vertex}
