# Supplementary material for: Specification and Implementation of Replicated List: The Jupiter Protocol Revisited
Source: arXiv:1708.04754 source file (2018-11-12)
Supplement: Supplementary file 2 [file appendix-djupiter-proof.tex]

% \section{Proofs for Section~\ref{section:djupiter}}    \label{section:appendix-djupiter}
\section{Distributed \jupiter{} Protocol}  \label{section:djupiter}

By orthogonally integrating the $n$-ary ordered state space
with a distributed scheme to totally order operations,
we further extend \cjupiter{} to a distributed setting.

Recall that the construction of $n$-ary ordered state space at each replica is
determined by the schedule of operations,
namely the causal and total orderings on operations.
Being distributed, the \djupiter{} (Distributed \jupiter{}) protocol
relies on an atomic broadcast~\cite{Defago:CSUR04, Attiya:Book04} to totally order operations.
Taking into account the requirement of preserving causality,
\djupiter{} assumes a causal atomic broadcast service~\cite{Attiya:Book04, Attiya:PODC16}
and behaves as \cjupiter{} with two exceptions:

%%%%%%%%%% the DCSS protocol %%%%%%%%%%
\begin{enumerate}
  \item In the case of a replica generating an operation $o$,
    the replica finally broadcasts $o$ to all replicas (including itself),
    utilizing the causal atomic broadcast service.
  \item Each replica receives and processes operations in the order
    enforced by the causal atomic broadcast service,
    ignoring the operations it generates.
\end{enumerate}
%%%%%%%%%% the DCSS protocol %%%%%%%%%%

\djupiter{} is a \emph{simulation} of \cjupiter{},
by replacing the central server in \cjupiter{} with an atomic broadcast service.
Thus, it also satisfies the weak list specification $\wlspec{}$.

%%%%%%%%%% prop:simulation %%%%%%%%%%
\begin{prop}[Simulation]    \label{prop:simulation}
  Let $\protinmath = \set{R_1, \ldots, R_n, S}$ be the \emph{\cjupiter{}} protocol
  running on a client/server system with $n$ clients $R_1, \ldots, R_n$ and a server $S$.
  Let $\protinmath' = \set{R'_1, \ldots, R'_n}$ be the \emph{\djupiter{}} protocol
  running on a distributed system with $n$ replicas.
  Then $\protinmath'$ is a simulation of \prot{} in the sense that
  for any execution $\alpha'$ of $\protinmath'$,
  there exists an execution $\alpha$ of \prot{} such that
  % $\alpha|_{R_i}^{\doe} = \alpha'|_{R'_i}^{\doe}\, , 1 \leq i \leq n$.
  \begin{equation*}
    \alpha|_{R_i}^{\doe} = \alpha'|_{R'_i}^{\doe}\, , \quad 1 \leq i \leq n.
  \end{equation*}
\end{prop}
%%%%%%%%%% prop:simulation %%%%%%%%%%
% \subsection{Proof for Proposition~\ref{prop:simulation} (Simulation)}

\begin{proof}
  Given an execution $\alpha'$ of $\protinmath'$,
  we construct an execution $\alpha$ of \prot{}
  satisfying $\alpha|_{R_i}^{\doe} = \alpha'|_{R'_i}^{\doe}$ as follows.

  Set $R_i = R'_i$, for $i = 1 \twodots n$.
  Execution $\alpha$ differs from $\alpha'$ in that:
  \begin{itemize}
    \item Instead of broadcasting a locally generated operation $o$,
      a replica sends $o$ to the server $S$.
    \item The server $S$ receives operations in the total order
      enforced by the causal atomic broadcast service in $\alpha'$.
      Furthermore, the server $S$ receives an operation $o$, say, from $R_i$, at some moment
      between $o$ is broadcast by $R'_i$ and $o$ is received by the first replica in $\alpha'$.
      % according to the causal atomic broadcast service.
    \item The server $S$ redirects these operations to all replicas in FIFO order.
    \item Each replica $R_i$ receives operations at the moment $R'_i$ does in $\alpha'$,
      and ignores the operations it generates.
  \end{itemize}
\end{proof}
