# Supplementary material for: Specification and Implementation of Replicated List: The Jupiter Protocol Revisited
Source: arXiv:1708.04754 source file (2018-11-12)
Supplement: Supplementary file 3 [file appendix-cjupiter-property.tex]

%%%%%%%%%%%%%%%%%%%%%%%%%%%%%%
\subsection{Properties of \cjupiter}  \label{ss:appendix-cjupiter-property}

Since the operations associated with the edges
from the same vertex in an $n$-ary ordered state space are pairwise concurrent by `$\parallel$'
and there are $n$ clients in total, we have

%%%%% lemma:n-ary %%%%%
\begin{lemma}[$n$-ary]  \label{lemma:n-ary}
  In \emph{\cjupiter{}}, each vertex in an $n$-ary ordered state space has at most $n$ child vertices. % (hence the name ``$n$''-ary).
\end{lemma}
%%%%% lemma:n-ary %%%%%

By \textsc{xForm}, the edges labeled with the operations with the same $oid$ are ``parallel''
(Figure~\ref{fig:xform-ot}). 
Therefore,

%%%%%%%%%%%%%%% lemma:simple-path %%%%%%%%%%%%%%%
\begin{lemma}[Simple Path]  \label{lemma:simple-path}
  Let $P_{v_1 \leadsto v_2}$ be a path 
  from vertex $v_1$ to vertex $v_2$ in an $n$-ary ordered state space.
  Then, there are no duplicate operations (in terms of their $oid$s)
  along the path $P_{v_1 \leadsto v_2}$.
  We call such a path a simple path.
\end{lemma}
%%%%%%%%%%%%%%% lemma:simple-path %%%%%%%%%%%%%%%

The operation sequence with which an operation transforms \emph{at the server}
can be characterized as follows. 

%%%%%%%%%%%%%%% lemma:cjupiter-ot-server %%%%%%%%%%%%%%%
\begin{lemma}[\cjupiter{} OT Sequence] \label{lemma:cjupiter-ot-server}
  In \emph{\textsc{xForm}} of \emph{\cjupiter{}}, 
  the operation sequence $L$ (may be empty) with which an operation $op$ transforms at the server
  consists of the operations that are both totally ordered by `$\prec_{s}$' before 
  and concurrent by \emph{`$\parallel$'} with $op$.
  Furthermore, the operations in $L$ are totally ordered by `$\prec_{s}$'.
\end{lemma}
%%%%%%%%%%%%%%% lemma:cjupiter-ot-server %%%%%%%%%%%%%%%

\input{appendix/proof-cjupiter-ot-sequence}
