# Supplementary material for: Specification and Implementation of Replicated List: The Jupiter Protocol Revisited
Source: arXiv:1708.04754 source file (2018-11-12)
Supplement: Supplementary file 4 [file proof-djupiter-simulation.tex]

% \subsection{Proof for Proposition~\ref{prop:simulation} (Simulation)}

\begin{proof}
  Given an execution $\alpha'$ of $\protinmath'$,
  we construct an execution $\alpha$ of \prot{}
  satisfying $\alpha|_{R_i}^{\doe} = \alpha'|_{R'_i}^{\doe}$ as follows.

  Set $R_i = R'_i$, for $i = 1 \twodots n$.
  Execution $\alpha$ differs from $\alpha'$ in that:
  \begin{itemize}
    \item Instead of broadcasting a locally generated operation $o$,
      a replica sends $o$ to the server $S$.
    \item The server $S$ receives operations in the total order
      enforced by the causal atomic broadcast service in $\alpha'$.
      Furthermore, the server $S$ receives an operation $o$, say, from $R_i$, at some moment
      between $o$ is broadcast by $R'_i$ and $o$ is received by the first replica in $\alpha'$.
      % according to the causal atomic broadcast service.
    \item The server $S$ redirects these operations to all replicas in FIFO order.
    \item Each replica $R_i$ receives operations at the moment $R'_i$ does in $\alpha'$,
      and ignores the operations it generates.
  \end{itemize}
\end{proof}
